# Supplementary material for: A Laplace-inspired Distribution on SO(3) for Probabilistic Rotation Estimation
Source: arXiv:2303.01743 source file (2023-03-03)
Supplement: Supplementary file 1 [file noise_inject.tex]

\ree{
\section{Experiments on ModelNet10-SO3 Dataset with Outlier  Injections}
To further demonstrate the robustness of our distribution, we manually inject outliers to the perfectly labeled synthetic dataset and compare Rotation Laplace distribution with matrix Fisher distribution. 
Specifically, we randomly choose 1\%, 5\%, 10\% and 30\% images from the training set of ModelNet10-SO3 dataset respectively, and apply a random rotation in $\SO$ to the given ground truth. Thus, the chosen images become outliers in the dataset due to the perturbed annotations. We fix the processed dataset for different methods.

The results on the perturbed dataset are shown in Table \ref{tab:noise} and Figure \ref{fig:noise}, where our method consistently outperforms matrix Fisher distribution under different levels of perturbations. More importantly, as shown in Figure \ref{fig:noise}, our method clearly better tolerates the outliers, resulting in less performance degradation and remains a reasonable performance even under intense perturbations. For example, Acc@30$^\circ$ of matrix Fisher distribution greatly drops from 0.751 to 0.467 with 30\% outliers, while that of our method merely goes down from 0.770 to 0.700, which shows the superior robustness of our method.
}

\begin{table}[t]
  \centering
  \fontsize{7.8}{9.5}\selectfont
  \caption{\ree{Comparisons on the perturbed ModelNet10-SO3 dataset where random outliers are injected.}}
    \begin{tabular}{clcccccc}
    \toprule
        Outlier Inject  &  Method     & Acc@3$^\circ$$\uparrow$ & Acc@5$^\circ$$\uparrow$ & Acc@10$^\circ$$\uparrow$ & Acc@15$^\circ$$\uparrow$ & Acc@30$^\circ$$\uparrow$ & Med.($^\circ$)$\downarrow$ \\
    \midrule
    
    \multirow{2}[0]{*}{0\%} 
    & \cite{mohlin2020probabilistic}    &  0.164& 0.389 &  0.615 &  0.684&  0.751&   17.9 \\
    & Rotation Laplace                  &  \textbf{0.446}  & \textbf{0.613}  &  \textbf{0.714}  &  \textbf{0.741}  &  \textbf{0.770} & \textbf{12.2}   \\
    \midrule
    \multirow{2}[0]{*}{1\%} 
    & \cite{mohlin2020probabilistic}    &  0.141    &	0.336&	0.589&	0.664&	0.740&	20.5\\
    & Rotation Laplace                  &  \textbf{0.429}&	\textbf{0.601}&	\textbf{0.711}&	\textbf{0.739}&   \textbf{0.769}	 &\textbf{12.4} %
    \\
    \midrule
    \multirow{2}[0]{*}{5\%} 
    & \cite{mohlin2020probabilistic}    &  0.0818&	0.229&	0.501&	0.605&	0.711&	24.8 \\
    & Rotation Laplace                  &   \textbf{0.368}&	\textbf{0.561}&	\textbf{0.693}&	\textbf{0.727}&	\textbf{0.762}&	\textbf{12.6} \\
    \midrule
    \multirow{2}[0]{*}{10\%} 
    & \cite{mohlin2020probabilistic}    &   0.0493&	0.151&	0.403&	0.536&	0.677&	26.8\\
    & Rotation Laplace                  &   \textbf{0.329}&	\textbf{0.523}&	\textbf{0.668}&	\textbf{0.706}&	\textbf{0.747}&	\textbf{16.1}\\
    \midrule
    \multirow{2}[0]{*}{30\%} 
    & \cite{mohlin2020probabilistic}    &   0.0063&	0.0255&	0.126&	0.243&	0.467&	45.3\\
    & Rotation Laplace                  &   \textbf{0.151}&	\textbf{0.345}&	\textbf{0.565}&	\textbf{0.634}&	\textbf{0.700}&	\textbf{22.7}\\
    \bottomrule
    \end{tabular}%
  \label{tab:noise}%
\end{table}%

\begin{figure}[t]
    \centering
    \includegraphics[width=0.32\linewidth]{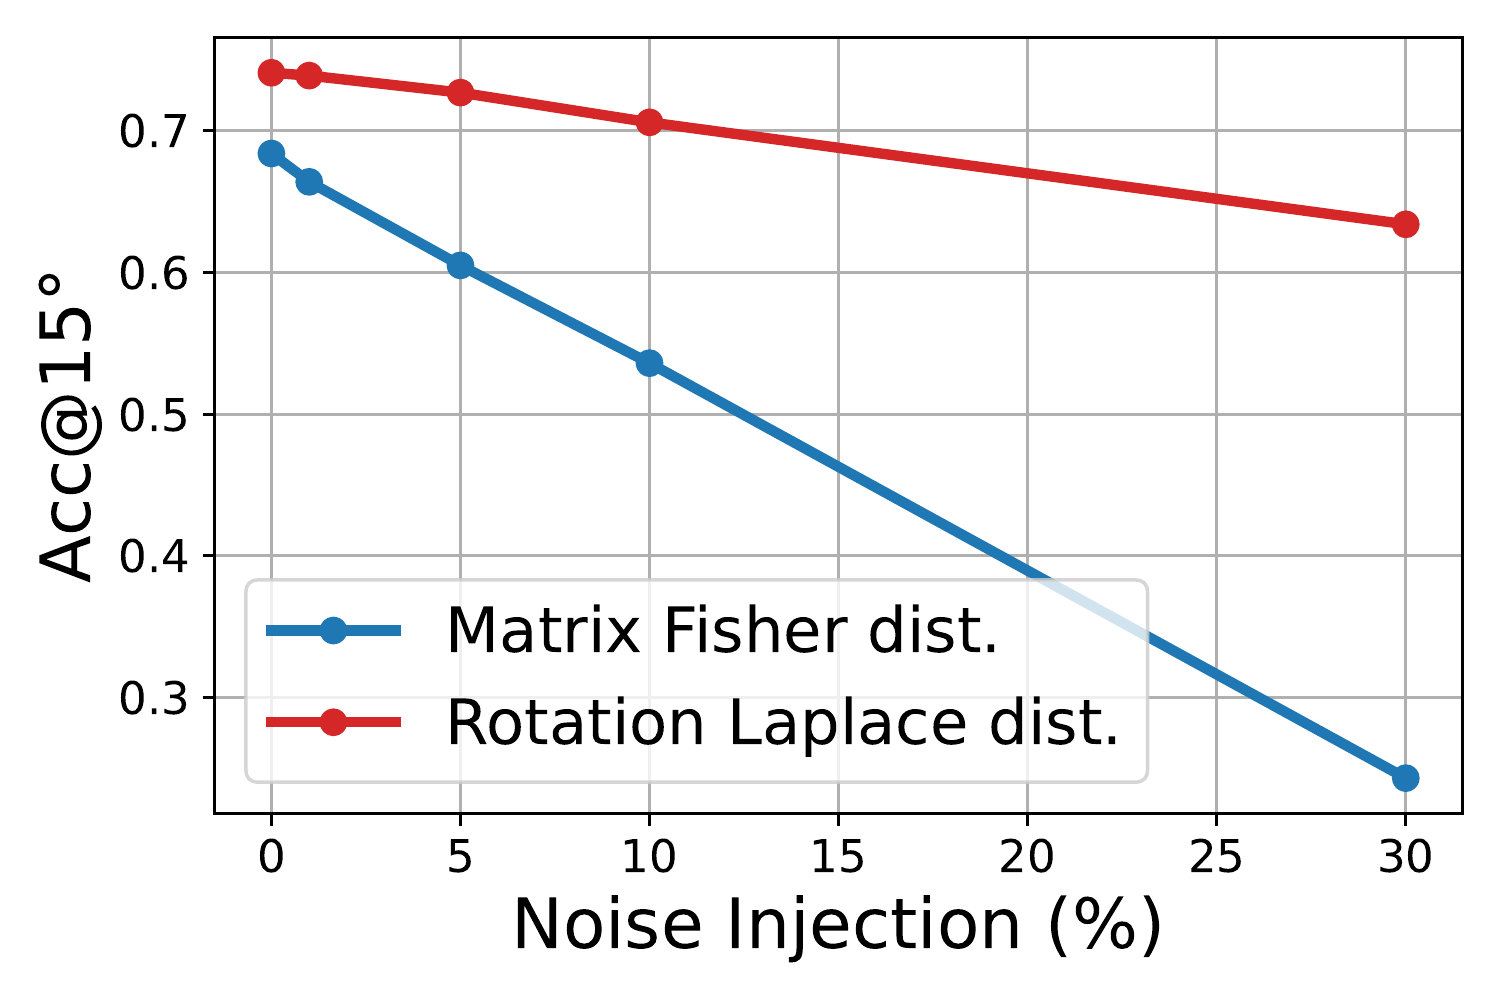}
    \includegraphics[width=0.32\linewidth]{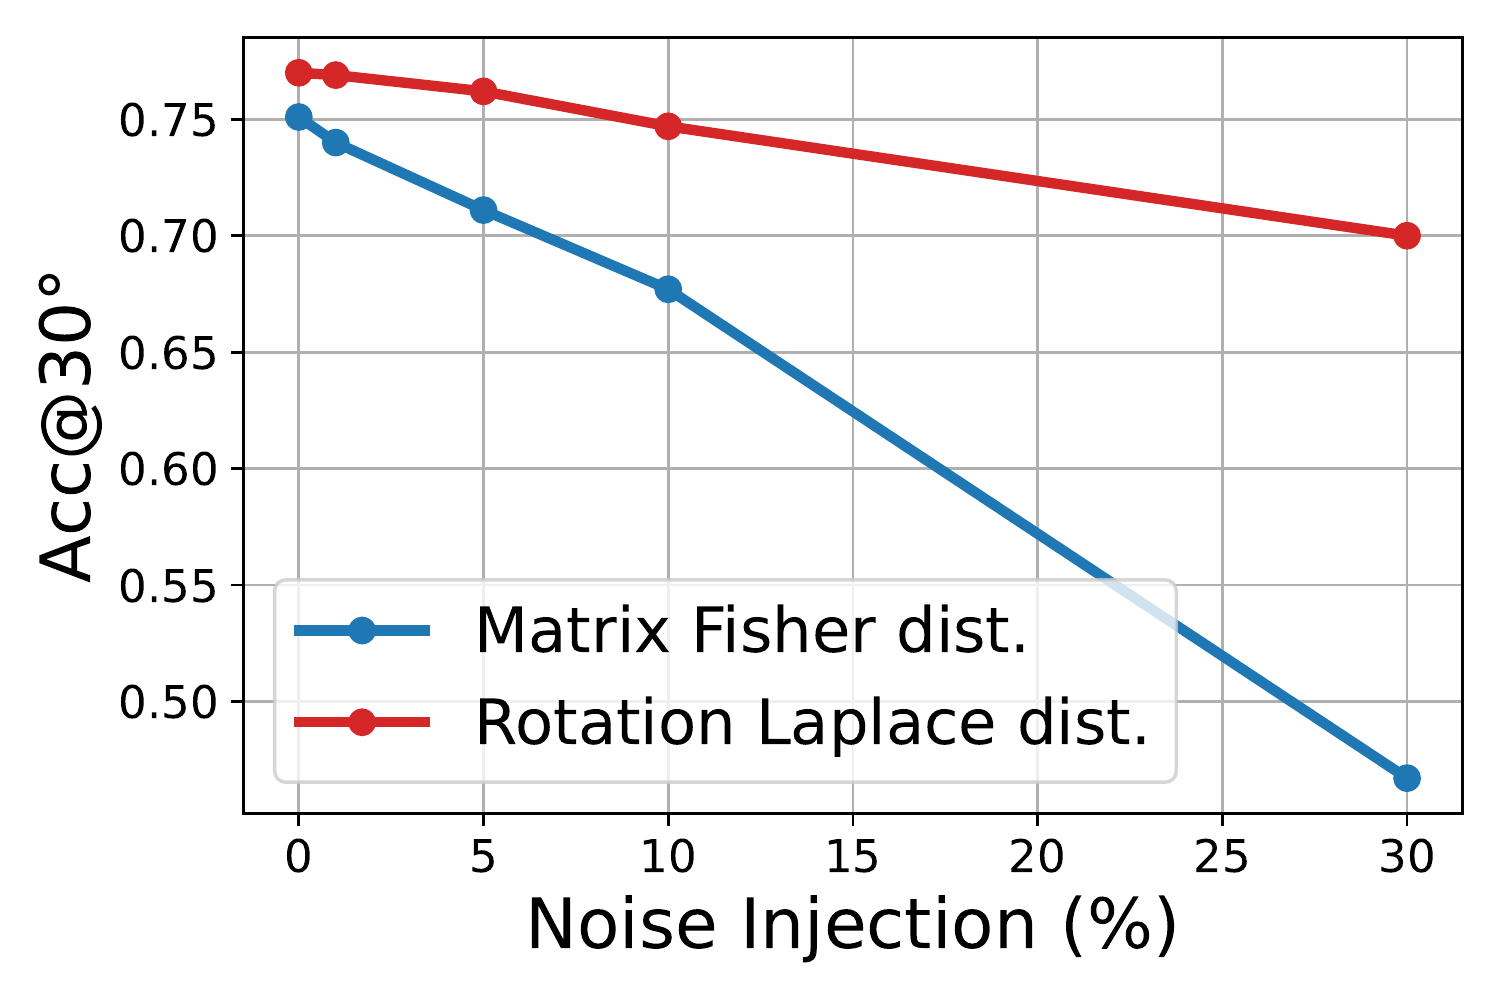}
    \includegraphics[width=0.32\linewidth]{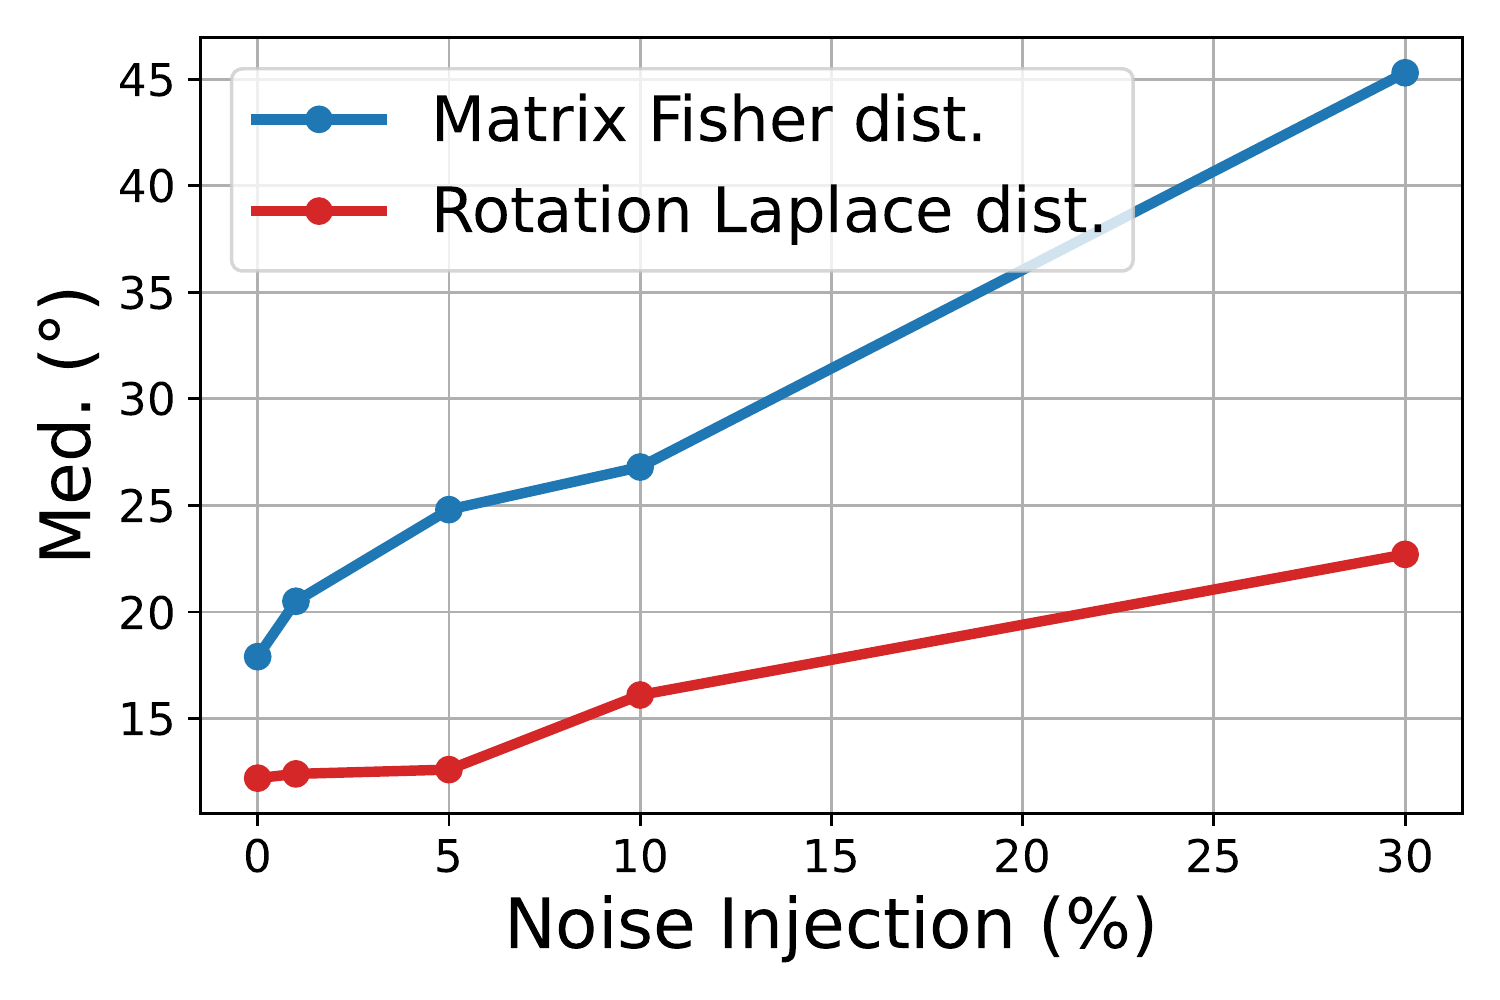}
    \caption{\ree{\textbf{Comparisons on the perturbed ModelNet10-SO3 dataset where random outliers are injected.}
    The horizontal axis is the percentage of perturbed images, and the vertical axis represents the corresponding metric.}}
    \vspace{-2mm}
	\label{fig:noise}
\end{figure}
