# Supplementary material for: A Laplace-inspired Distribution on SO(3) for Probabilistic Rotation Estimation
Source: arXiv:2303.01743 source file (2023-03-03)
Supplement: Supplementary file 2 [file supp_tab_noise.tex]

\begin{table}[t]
  \centering
  \fontsize{7.8}{9.5}\selectfont
  \caption{\ree{Comparisons on the perturbed ModelNet10-SO3 dataset where random outliers are injected.}}
    \begin{tabular}{clcccccc}
    \toprule
        Outlier Inject  &  Method     & Acc@3$^\circ$$\uparrow$ & Acc@5$^\circ$$\uparrow$ & Acc@10$^\circ$$\uparrow$ & Acc@15$^\circ$$\uparrow$ & Acc@30$^\circ$$\uparrow$ & Med.($^\circ$)$\downarrow$ \\
    \midrule
    
    \multirow{2}[0]{*}{0\%} 
    & \cite{mohlin2020probabilistic}    &  0.164& 0.389 &  0.615 &  0.684&  0.751&   17.9 \\
    & Rotation Laplace                  &  \textbf{0.446}  & \textbf{0.613}  &  \textbf{0.714}  &  \textbf{0.741}  &  \textbf{0.770} & \textbf{12.2}   \\
    \midrule
    \multirow{2}[0]{*}{1\%} 
    & \cite{mohlin2020probabilistic}    &  0.141    &	0.336&	0.589&	0.664&	0.740&	20.5\\
    & Rotation Laplace                  &  \textbf{0.429}&	\textbf{0.601}&	\textbf{0.711}&	\textbf{0.739}&   \textbf{0.769}	 &\textbf{12.4} %
    \\
    \midrule
    \multirow{2}[0]{*}{5\%} 
    & \cite{mohlin2020probabilistic}    &  0.0818&	0.229&	0.501&	0.605&	0.711&	24.8 \\
    & Rotation Laplace                  &   \textbf{0.368}&	\textbf{0.561}&	\textbf{0.693}&	\textbf{0.727}&	\textbf{0.762}&	\textbf{12.6} \\
    \midrule
    \multirow{2}[0]{*}{10\%} 
    & \cite{mohlin2020probabilistic}    &   0.0493&	0.151&	0.403&	0.536&	0.677&	26.8\\
    & Rotation Laplace                  &   \textbf{0.329}&	\textbf{0.523}&	\textbf{0.668}&	\textbf{0.706}&	\textbf{0.747}&	\textbf{16.1}\\
    \midrule
    \multirow{2}[0]{*}{30\%} 
    & \cite{mohlin2020probabilistic}    &   0.0063&	0.0255&	0.126&	0.243&	0.467&	45.3\\
    & Rotation Laplace                  &   \textbf{0.151}&	\textbf{0.345}&	\textbf{0.565}&	\textbf{0.634}&	\textbf{0.700}&	\textbf{22.7}\\
    \bottomrule
    \end{tabular}%
  \label{tab:noise}%
\end{table}%
